# Supplementary material for: AdaEvo: Edge-Assisted Continuous and Timely DNN Model Evolution for Mobile Devices
Source: arXiv:2309.15500 source file (2023-10-25)
Supplement: Supplementary file 1 [file appendix.tex]

\appendix
\newrev{
\section{Appendix}
% The way of calculating the grouping number K is mainly related to the distribution of the model evolving urgency $\lambda_{i}$ and the strategy of task grouping. 
The determination of the grouping number K depends primarily on two factors: the distribution of the model evolving urgency, denoted as $\lambda_{i}$, and the strategy employed for task grouping
% \TODO{revise this sentence}
Specifically, as we mentioned in \S~\ref{sec:searchspace}, we approximate the distribution of $\lambda_{i}$ as a normal distribution with $\frac{1}{2}(\lambda_{max}+\lambda_{min})$ as the mean and $\sigma^{2}$ as the variance. As shown in Figure~\ref{fig:number} in the paper, $\beta$ is the model evolving urgency range length of the last group.
    For a normal distribution with mean $\mu$ and variance $\sigma^{2}$, its probability density function is
    \begin{equation}
    \quad f(x) = \frac{1}{\sigma\sqrt{2\pi}}exp[-\frac{(x-\mu)^{2}}{2\sigma^{2}}]
   \label{eqn:normal_ditribution}
\end{equation}
    The probability that x falls within $[\mu-a,\mu+a]$ can be expressed by the error function~\cite{bib:error_function}:
    \begin{equation}
    \quad P \left\{ |x-\mu|\leq a\right\} = \int_{-a}^{a}f(x)dx = erf(\frac{a}{\sqrt{2}\sigma})
   \label{eqn:normal_ditribution}
\end{equation}
Based on the above analysis, we can calculate the probability that the task appears between group2 and groupK-1. Due to the symmetry of the normal distribution, the model evolving urgency ranges of group1 and groupK are both $\beta$. Therefore, the probability that the task appears between group2 and groupK-1 can be regarded as the probability that x is located in $[\frac{1}{2}(\lambda_{max}+\lambda_{min})-\frac{1}{2}(\lambda_{max}-\lambda_{min}-2\beta),\frac{1}{2}(\lambda_{max}+\lambda_{min})+\frac{1}{2}(\lambda_{max}-\lambda_{min}-2\beta])$, which is $erf(\frac{\frac{1}{2}(\lambda_{max}-\lambda_{min})-\beta}{\sqrt{2}\sigma})$.
Besides, since we adopt the equal task probability grouping method, the probability of tasks appearing in each group is the same. And, for the probability density function, $\int_{-\infty}^{+\infty}f(x)dx = 1$.
Therefore, the probability that the task appears in group2 to gourp K-1 can also be expressed as $\frac{K-2}{K}*\int_{-\infty}^{+\infty}f(x)dx = \frac{K-2}{K}$. We can establish the equation and get the formula for grouping number K (Equation~\ref{equ:m} in the paper):
    \begin{equation}
    \quad \frac{K-2}{K} = erf(\frac{\frac{1}{2}(\lambda_{max}-\lambda_{min})-\beta}{\sqrt{2}\sigma})
   \label{eqn:normal_ditribution}
\end{equation}
K needs to be an integer, so we handle it with the rounding function $int()$.
In addition, we need to limit the number of tasks and the model evolving urgency range length of each group to obtain a good search space. 
Since we use equal task probability grouping, the number of tasks in each group is roughly the same. 
Based on the probability of group 2 to group K-1 calculated by the error function and the symmetry of the normal distribution, we can get the probability that the task appears in group1. 
We set the minimum number of tasks for each group to limit the maximum value of K:
\begin{equation}
    \frac{1}{2}N[1-erf(\frac{\frac{1}{2}(\lambda_{max}-\lambda_{min})-\beta}{\sqrt{2}\sigma})]\geq n_{min}
\end{equation}
Where N denotes the maximum number of requests the edge server can handle concurrently at most. 
Depending on the characteristics of the normal distribution, the range length of gourp1 and groupK is the largest.
And we limit it, thereby limiting the maximum number of tasks in each group and the minimum value of K of the group :
\begin{equation}
    \beta \leq \varepsilon
\end{equation}
Where $\varepsilon$ indicates the threshold of acceptable model evolving urgency range length.
}
